# Supplementary material for: Decaf: Improving Neural Decompilation with Automatic Feedback and Search
Source: arXiv:2605.11501 source file (2026-05-12)
Supplement: Supplementary file 1 [file GenAiUse.tex]

\section{Generative AI Usage}

AI tools were used to assist programming the project: Cursor and Claude were used to develop code. Code development was done rigorously to ensure that crucial components of the project such as the validity of functional correctness experiments were correct and consistent throughout the development of our project. We developed and maintained a large amount of functionality tests to ensure that changes to our code base would not change how we fundamentally evaluate our code. We wrote a very large degree of the code and performed a large degree of manual verification and re-reading of ai-assisted code. 

Our paper was written by our authors. Claude was used for grammar and typo checking and to suggest rephrasing sentences for clarity and flow. Claude was also used to to help brainstorm and draft an initial Ethical Considerations section which we then read, omitted inaccuracies and misrepresentations, adapted in our language, and re-framed to fit our paper.
