# Supplementary material for: Decaf: Improving Neural Decompilation with Automatic Feedback and Search
Source: arXiv:2605.11501 source file (2026-05-12)
Supplement: Supplementary file 2 [file ethics.tex]

\section{Ethical Considerations}
\label{sec:ethics}

\noindent\textbf{Stakeholders}. We identify four primary stakeholder groups: (1) security practitioners and reverse engineers who benefit from improved decompilation tools, (2) software developers and companies whose proprietary binaries could be more easily reverse-engineered, (3) the broader research community, and (4) the authors and research team.

\noindent\textbf{Dual-Use Considerations}. Decompilation is an inherently dual-use technology. Improved decompilation directly benefits defensive security tasks, including malware analysis, vulnerability discovery, legacy software maintenance, and compliance auditing, which constitute the primary intended use of our work. However, the same capabilities could lower the barrier for adversarial reverse engineering of proprietary software or aid in circumventing intellectual property protections. We believe the defensive benefits substantially outweigh the adversarial risks for several reasons. First, well-resourced adversaries already have access to sophisticated commercial decompilation tools (e.g., Hex-Rays); our work primarily closes the gap for defenders using freely available tools like Ghidra. Second, decompilation has been an active area of both academic and industrial research for over three decades, and our contributions are incremental improvements to an established capability rather than a qualitatively new threat. Third, legal frameworks such as the DMCA and CFAA already govern the contexts in which reverse engineering is permissible; our tools do not circumvent these protections.

\noindent\textbf{Mitigated Harm: Arbitrary code execution}. Our methodology requires compiling and executing hundreds of thousands of LLM-generated programs. To mitigate the risk of malicious or unintended side effects, all generated code was compiled and executed within isolated, containerized environments with no network access and restricted filesystem permissions. Programs were terminated after fixed time and memory limits. Our Dockerfile and environment setup scripts are included with our artifacts.

\noindent\textbf{Mitigated Harm: Reproducibility and defensive access}. To ensure our contributions primarily benefit the defensive security community, we plan to release our models, data, and evaluation infrastructure openly, rather than restricting access to well-resourced actors who could independently develop similar capabilities.

\noindent\textbf{Risk: Benchmark limitations as a false sense of security}. Our evaluation relies on \Exebench test cases to approximate functional correctness. Insufficient test coverage may admit false positives, potentially giving users unwarranted confidence in a decompilation's correctness. We acknowledge this limitation in \Cref{sec:threats-to-validity} and caution practitioners to treat \Decaf outputs as aids to understanding rather than verified equivalences.

\noindent\textbf{Risk: Lack of Generalization to malicious binaries}. Our system is trained and evaluated on benign open-source code. We have not evaluated its behavior on obfuscated or adversarially crafted binaries, therefore its reliability in real-world malware analysis scenarios remains unvalidated. In our writing we do not make claims about the ability to generalize to malicious code. 

% \noindent\textbf{Team Wellbeing}. The computational demands of our experiments, including training large models for multiple weeks and executing large-scale inference, were conducted on institutional compute infrastructure. No team members were exposed to harmful content or placed at legal risk during the course of this research.

% \noindent\textbf{Decision}. \medskip
We believe the benefits of publishing this work, including advancing the state of decompilation for defensive security, contributing reproducible artifacts and methodology to the research community, and demonstrating a general paradigm for improving neural program analysis with automatic feedback, outweigh the potential increase in adversarial capability. We plan to release our models and evaluation infrastructure to enable reproducibility and to allow the defensive security community to directly benefit from our contributions.
