# Supplementary material for: Decaf: Improving Neural Decompilation with Automatic Feedback and Search
Source: arXiv:2605.11501 source file (2026-05-12)
Supplement: Supplementary file 3 [file open_science.tex]

% Open Science Appendix - include with: \input{paper/open_science}

\section{Open Science}

\noindent\textbf{Artifact Repository:} \url{https://anonymous.4open.science/r/decaf-ccs/}

\smallskip
\noindent\textit{Note:} Models are hosted on HuggingFace under an anonymized account due to size (e.g. $\sim$83GB \DecafLLM, $\sim$120GB \DecafReranker). We request reviewers not access commit history or external links to prevent deanonymization. The provided download script will allow downloading of the data and models without the risk of de-anonymization. We were not aware of any reasonable alternative to this to allow sharing of our models and data in line with the Open Science requirement. 

% \smallskip
% \noindent\textbf{Artifacts Released:}
% \textbf{Models:} Fine-tuned \DecafLLM and \DecafReranker.

% \smallskip
% \textbf{Data:} Data for evaluation.

\smallskip
\noindent\textbf{Environment Setup:}
We recommend opening the repository as a Dev Container in VS Code. Edit \texttt{.devcontainer/devcontainer.json} to mount your storage directory on the host machine. After building the container, run \texttt{.devcontainer/conda\_install.sh} to install all dependencies. For training dependencies, run \linebreak \texttt{.devcontainer/trainer\_dependencies.sh}. Additionally, a \texttt{HF\_TOKEN} from HuggingFace will need to be created and added to the environment and the \texttt{\.dotenv} file in the project to authorize HuggingFace. 

\smallskip
\noindent\textbf{Key Scripts:}\\
\texttt{scripts/download.sh} -- download models/data from HuggingFace\\
\texttt{scripts/inference.py} -- LLM inference (vLLM) to sample from the LLMs for decompilation.\\
\texttt{scripts/evaluator.py} -- Evaluation for LLM generated decompilations: compilation, execution, edit distance, etc. \\
\texttt{scripts/eval\_rerank.py} -- reranking using the different reranking methodologies. \\
\texttt{src/utils/exebench.py} -- core utility for compiling, executing, disassembling, and evaluating \Exebench examples. \\
\texttt{src/training/trainer.py} -- Supervised Fine-Tuning training 

\smallskip
\noindent\textbf{Experiment Drivers:}
The \texttt{scripts/merged\_test\_set\_experiments/} directory contains shell scripts for running all experiment configurations across the different models evaluated for inference, evaluation, and reranking.

\smallskip
\noindent\textbf{Juliet Reproduction:}
After \texttt{./scripts/download.sh -{}-all}, run \linebreak
\texttt{./scripts/juliet/run\_juliet\_pipeline.sh} for the end-to-end pipeline,
or \texttt{./scripts/juliet/run\_juliet\_pipeline.sh analyze} to re-run just
the CodeQL analysis and metric aggregation against reranked outputs.

\smallskip
\noindent\textbf{Configurations:}\\
\texttt{configs/test\_experiments/} -- inference, eval, rerank configs\\
\texttt{configs/training/} -- model training configs

\smallskip
\noindent\textbf{Testing:} To verify the environment setup, run \texttt{pytest tests/ -{}-ignore=tests/models/ -v}. This validates core functionality (compilation, execution, distance metrics) without requiring GPU resources.

\smallskip
\noindent\textbf{Reproduce:} Run \texttt{./scripts/download.sh -{}-all} to fetch models and data, then execute the appropriate driver scripts or manually run the scripts with affiliated configs.
